# Supplementary material for: Domain Generalization via Causal Adjustment for Cross-Domain Sentiment Analysis
Source: arXiv:2402.14536 source file (2024-02-22)
Supplement: Supplementary file 1 [file 070appendix.tex]

\section{Appendix A}
\label{sec:appendix}
%Codition of backdoor adjustment
(Identifiablity) The Backdoor adjustment formulation cannot be used arbitrarily, the adjustment variable $D$ should satisfies the backdoor criterion relative to $X$ and $Y$ if:

%Given a DAGs $G$, a set of nodes $Z$, and a pair of nodes, namely $X$ and $Y$, we say that $Z$ satisfies the backdoor criterion relative to $X$ and $Y$ if:
\begin{itemize}
\item[$\bullet$] No node in $D$ is a descendant of $Y$.
\item[$\bullet$] Every path between $X$ and $Y$ that contains an arrow pointing to $X$ is blocked by $D$.
\end{itemize}

In our SCM, we consider the adjustment between $M_{inv}$ and $Y$, and the adjustment varivable is the domain $D$.
Fortunately, the domain $D$ satisfies the backdoor criterion: (1) sentiment label $D$  obviously cannot be the factor of domain and therefore is not the descendant of $Y$. (2) "path between $M_{inv}$ and $Y$ that contains an arrow pointing to $M_{inv}$" is the backdoor path between $M_{inv}$ and $Y$. The two backdoor path in our SCM, i.e. $M_{inv} \leftarrow D \rightarrow Y$ and $M_{inv} \leftarrow D \leftarrow M_{spc} \rightarrow Y$ both can be blocked by $D$. It means that when condition on $D$ as the backdoor adjustment formula, $D$ elimate the correlation between $M_{inv}$ and $Y$. 

So the causal effect between $M_{inv}$ and $Y$ is identifiable and can be formulated as,
$$ P (Y \mid do(M_{inv})) = \sum_{D} P (Y \mid M_{inv}, D)P (D) $$
From the adjustment above, The pure causal effect $P (Y \mid do(M_{inv}))$ is extracted from the total effect $P (Y \mid M_{inv})$ by removing the spurious correlation caused by backdoor path.

%"contains an arrow pointing to M_inv" is the path like M_inv <--D-->Y (also called backdoor path), such a path may make M_inv and Y related but does not pass the causal effect generated by M_inv. "D blocks the path" means when condition on D as the backdoor adjustment formula, D elimate the correlation between M_inv and Y. 

%If $Z$ satisfies the backdoor criterion for $X$ and $Y$, the causal effect between $X$ and $Y$ is identifiable. The causal effect from $X$ to $Y$ can be formulated as,
%$$ P (Y \mid do(X)) = \sum_{Z} P (Y \mid X, Z)P (Z) $$
%%Notice $p(y \mid x) \neq p(y \mid do(x))$: %this do-notation is used in causal inference to indicate that an intervention has set $X = x$.
%%$do(\cdot)$ is used in causal inference to indicate that an intervention has set $X = x$.

\section{Appendix B}
\label{sec:appendix b}
We implement the model with PyTorch based on Hugging Face Transformer \footnote{\href{https://huggingface.co/bert-base-uncased}{https://huggingface.co/bert-base-uncased}.} and run them on the GPU(NVIDIA GTX 2080ti).
%For our $\mathcal{L}_\mathrm{invariant}$%specific hyper-parameters, $\alpha $ and $\beta$ are searched in $[0.1, 100]$. 
For DANN, the alpha is searched in \{0.1, 0.2, 0.5, 1\}. For Mixup, the mixup alpha is searched in \{0.1, 0.2\}. For GroupDRO, the groupdro eta is searched in \{0.001, 0.001, 0.1\}. For VREx, the lam and anneal iters are searched in \{0.3, 1, 10\} and \{100, 500\} respectively.

For the representation visualization, both settings are identical except for the input variations, with n\_components=2 and perplexity=100.

During the inference phase, the text representation is passed through the inv\_encoder and spc\_encoder to obtain invariant and specific representations respectively. These representations are then combined as a joint representation, and the probability from the joint classifier is used as the final result. The reason for setting it up this way during inference is that the information used is generic and applicable to any domain. This ensures strong generalization capabilities in scenarios where the test data is unseen.
